# Supplementary material for: Sculpting liquid crystal skyrmions with external flows
Source: arXiv:2303.12045 source file (2023-03-21)
Supplement: Supplementary file 1 [file SM.pdf]

# Supplemental Material: Sculpting liquid crystal skyrmions with external flows

Rodrigo C. V. Coelho,[1,2] Hanqing Zhao,[3] Mykola Tasinkevych,[1,2,4,5,*]
Ivan I. Smalyukh,[3,6,7,5,†] and Margarida M. Telo da Gama[1,2]

[1] *Centro de Física Teórica e Computacional, Faculdade de Ciências, Universidade de Lisboa, 1749-016 Lisboa, Portugal.*

[2] *Departamento de Física, Faculdade de Ciências, Universidade de Lisboa, P-1749-016 Lisboa, Portugal.*[‡]

[3] *Department of Physics and Soft Materials Research Center, University of Colorado Boulder, CO 80309, USA.*

[4] *SOFT Group, School of Science and Technology, Nottingham Trent University, Clifton Lane, Nottingham NG11 8NS, United Kingdom.*

[5] *International Institute for Sustainability with Knotted Chiral Meta Matter, Hiroshima University, Higashihiroshima 739-8511, Japan.*

[6] *Department of Electrical, Computer, and Energy Engineering and Materials Science and Engineering Program, University of Colorado, Boulder, CO 80309.*

[7] *Renewable and Sustainable Energy Institute, National Renewable Energy Laboratory and University of Colorado, Boulder, CO 80309, USA.*

(Dated: March 17, 2023)

This Supplemental Material provides additional figures to support the discussion in the main text.

* mykola.tasinkevych@ntu.ac.uk

† ivan.smalyukh@colorado.edu

‡ rcvcoelho@fc.ul.pt

TABLE I. Parameters used in the simulations, both in simulation and physical units. See the main text for definitions of these parameters.

| symbol | sim. units | physical units | description |
|---|---|---|---|
| $\rho$ | 1 | 1088 Kg/m$^3$ | density |
| $\Delta x$ | 1 | 0.625 $\mu$m | lattice spacing |
| $\Delta t$ | 1 | $10^{-8}$ s | time step |
| $L_1$ | $1.0226 \times 10^{-6}$ | $1.56 \times 10^{-12}$ J/m | $1^{st}$ elastic constant |
| $L_2$ | $2.3062 \times 10^{-6}$ | $3.52 \times 10^{-12}$ J/m | $2^{nd}$ elastic constant |
| $\Gamma$ | 0.474 | 12.14 Pa$^{-1}$s$^{-1}$ | rotational diffusivity |
| $\xi$ | 0.82 | 0.82 | alignment parameter |
| $a$ | 0.00256 | $0.01 \times 10^6$ J/m$^3$ | energy coefficient |
| $b$ | 0.208896 | $0.816 \times 10^6$ J/m$^3$ | energy coefficient |
| $c$ | 0.1152 | $0.45 \times 10^6$ J/m$^3$ | energy coefficient |
| $\nu$ | 0.909 | $3.550 \times 10^{-5}$ m$^2$/s | kinematic viscosity |
| $p$ | 16 | 10 $\mu$m | cholesteric pitch |
| $W_0$ | $1.2 \times 10^{-7}$ | $2.93 \times 10^{-7}$ J/m$^2$ | anchoring strength |
| $\chi$ | 0.0426 | $1.04 \times 10^{-9}$ N s/m | friction coefficient |

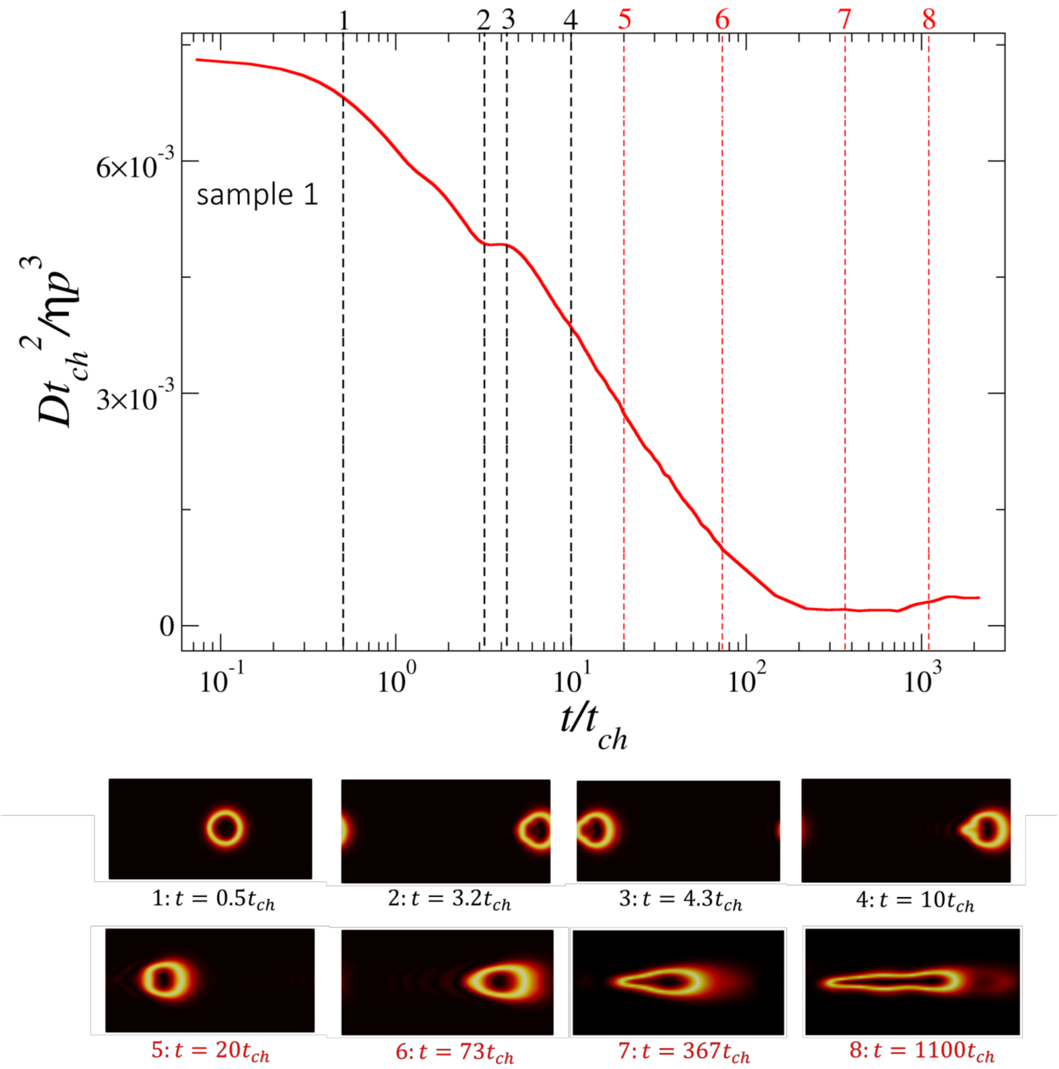


FIG. S1. Top: dissipation rate $D$ in Eq. 14 of the main text, as a function of time, at $\langle u \rangle = 14671.36\,\mu m/s$ (sample 1, $t_{ch} \approx 0.0007s$). The vertical dashed lines mark the times when the skyrmion configurations, depicted in the bottom panel, were taken. Times given by the black lines are in the scaling regime where data collapse of $\varepsilon(t/t_{ch})$ is observed, see Fig. 3(a). The flow proceeds from left to right.

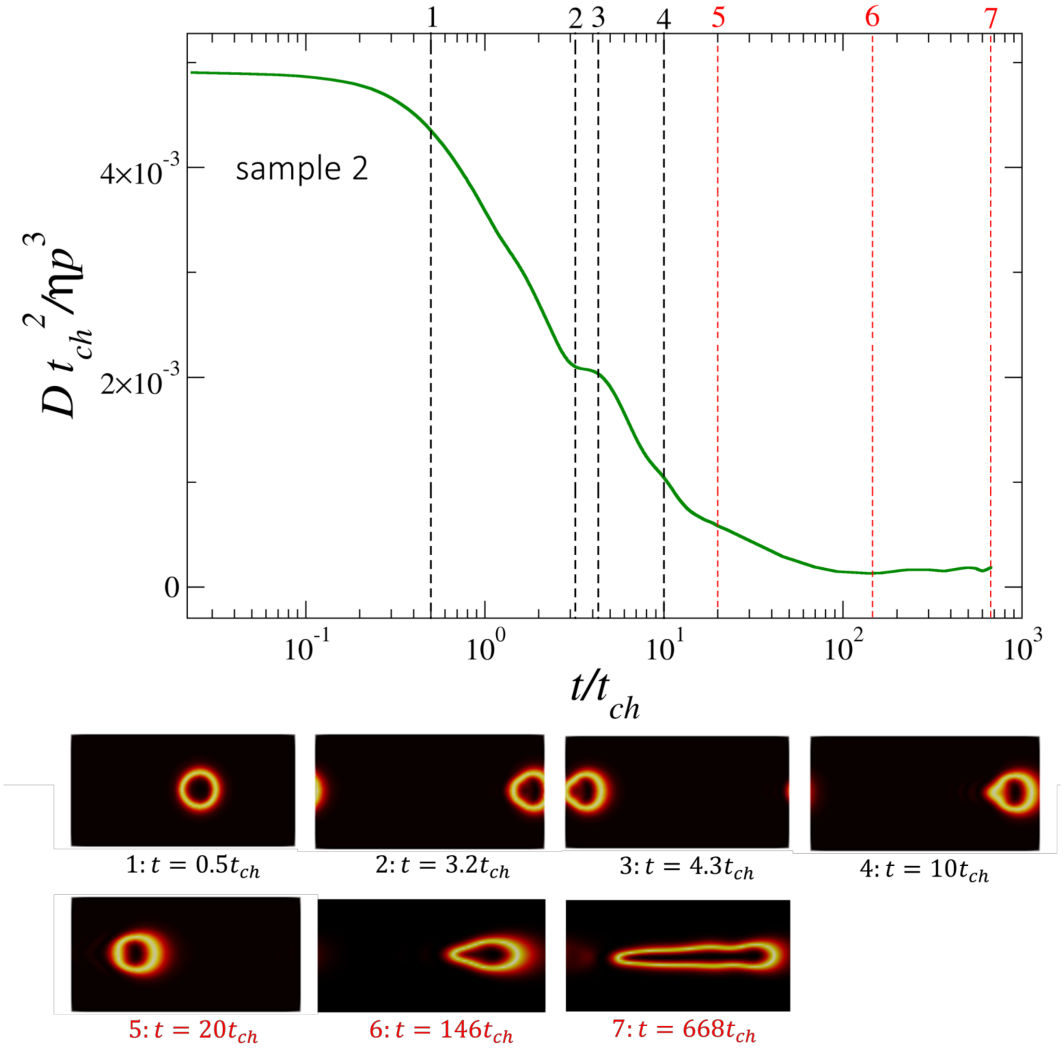


FIG. S2. Top: dissipation rate $D$ in Eq. 14 of the main text, as a function of time, at $\langle u \rangle = 4636.15\,\mu m/s$ (sample 2, $t_{ch} \approx 0.002s$). The vertical dashed lines mark the times when the skyrmion configurations, depicted in the bottom panel, were taken. Times given by the black lines are in the scaling regime where data collapse of $\varepsilon(t/t_{ch})$ is observed, see Fig. 3(a). The flow proceeds from left to right.

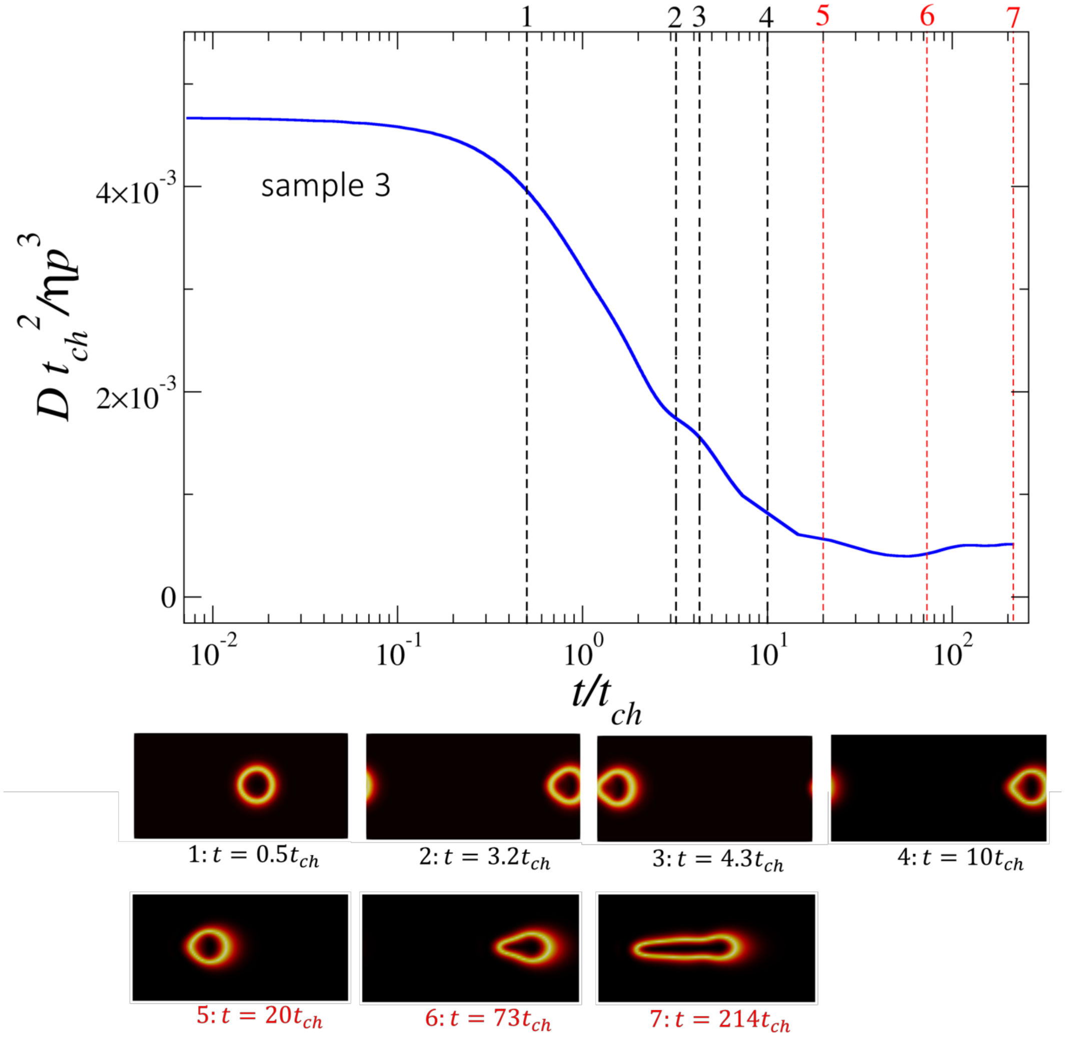


FIG. S3. Top: dissipation rate $D$ in Eq. 14 of the main text, as a function of time, at $\langle u \rangle = 1467.14\,\mu m/s$ (sample 3, $t_{ch} \approx 0.007s$). The vertical dashed lines mark the times when the skyrmion configurations, depicted in the bottom panel, were taken. Times given by the black lines are in the scaling regime where data collapse of $\varepsilon(t/t_{ch})$ is observed, see Fig. 3(a). The flow proceeds from left to right.

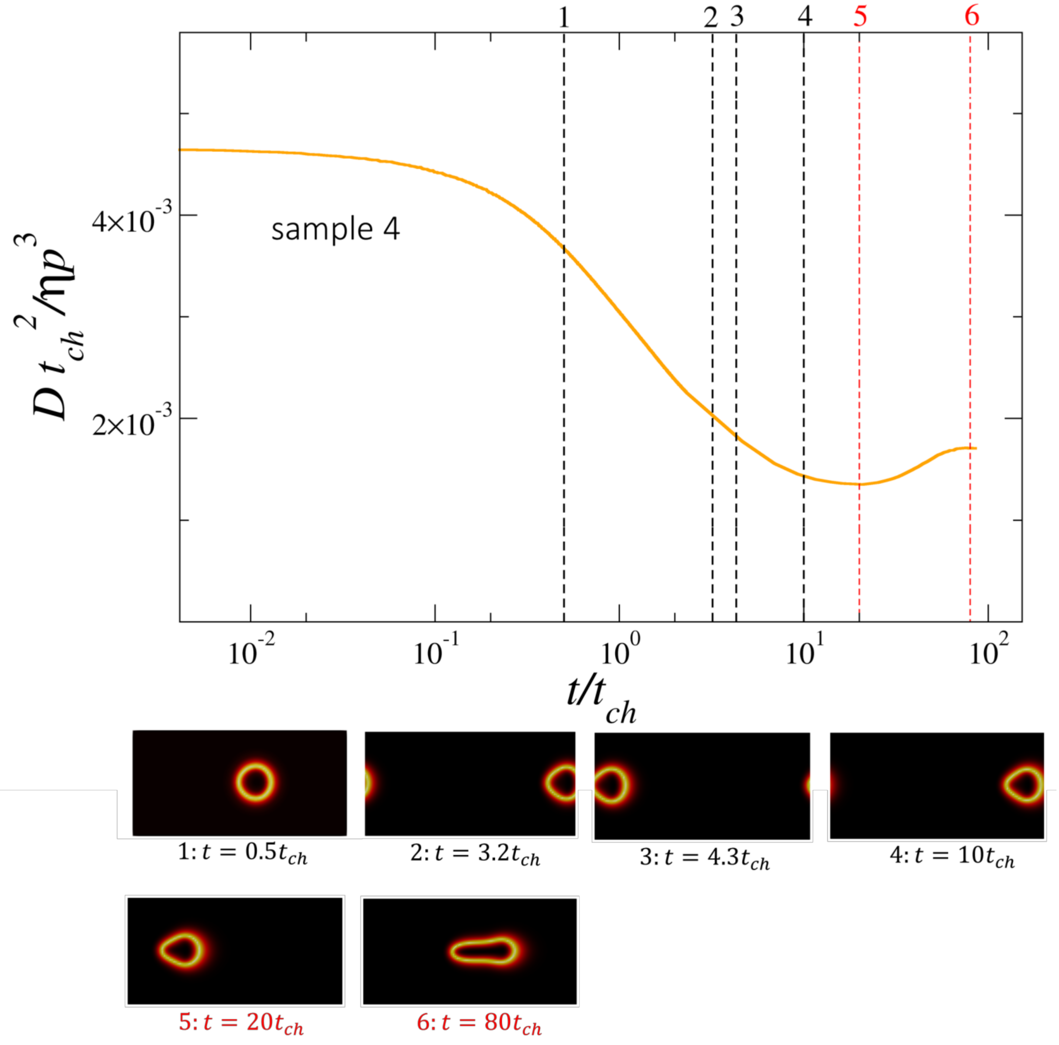


FIG. S4. Top: dissipation rate $D$ in Eq. 14 of the main text, as a function of time, at $\langle u \rangle = 463.62\,\mu m/s$ (sample 4, $t_{ch} \approx 0.02s$). The vertical dashed lines mark the times when the skyrmion configurations, depicted in the bottom panel, were taken. Times given by the black lines are in the scaling regime where data collapse of $\varepsilon(t/t_{ch})$ is observed, see Fig. 3(a). The flow proceeds from left to right.

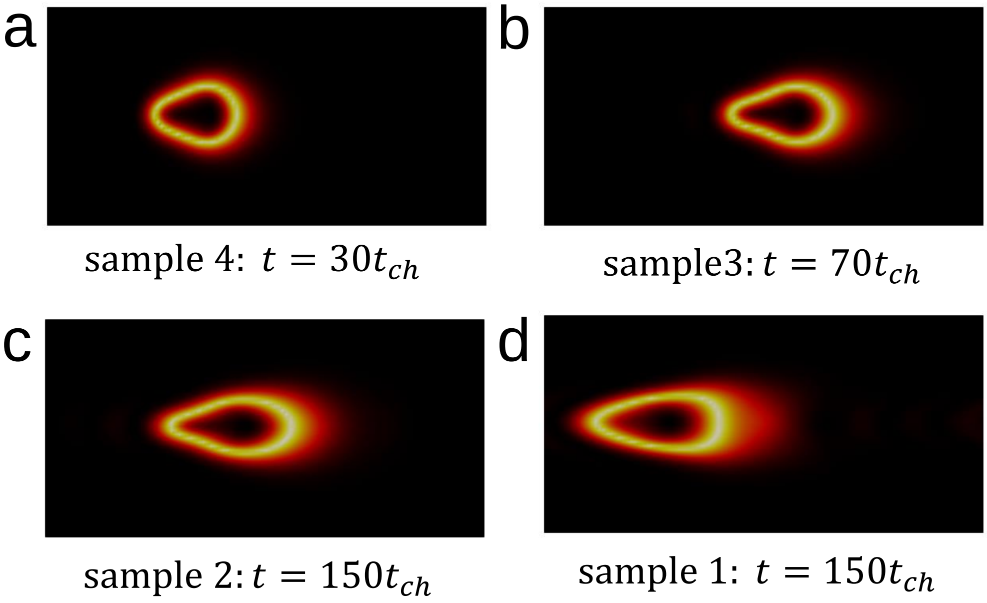


FIG. S5. Skyrmion configurations at the onset of the breakdown of the scaling behaviour of $\varepsilon(t/t_{ch})$: (a) sample 4, at $t = 30t_{ch}$; (b) sample 3, at $t = 70t_{ch}$; (c) sample 2, at $t = 150t_{ch}$. (d) For comparison the configuration of sample 1 at $t = 150t_{ch}$ is also shown.

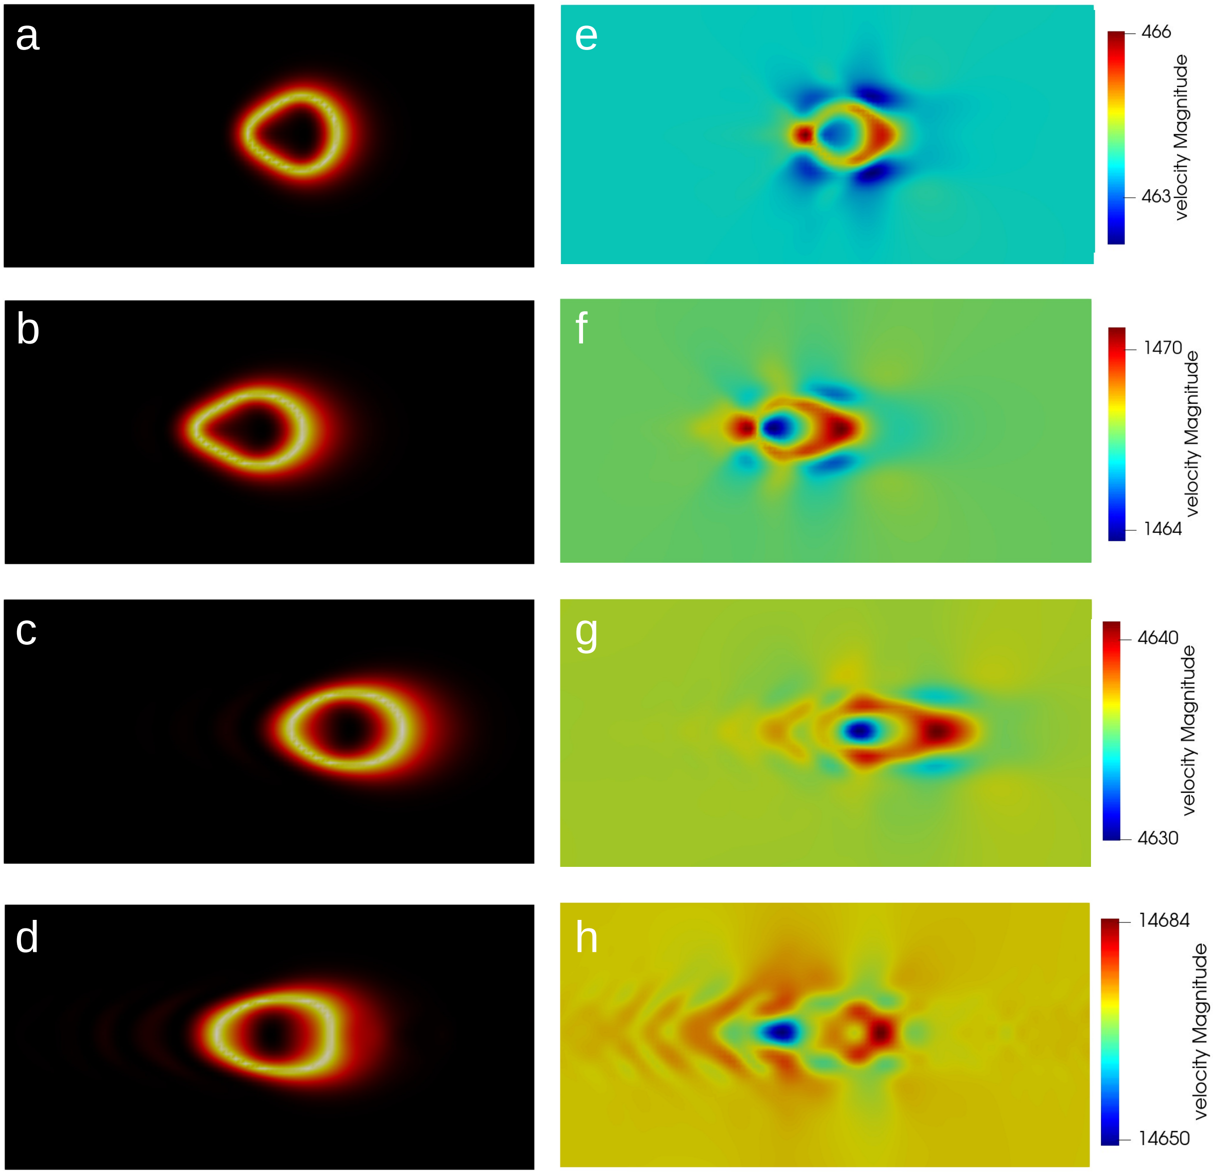


FIG. S6. (a)-(d) Skyrmion configurations obtained at $t \approx 50t_{ch}$ for (a) sample 4, $\langle u \rangle = 463.62\,\mu m/s$; (b) sample 3, $\langle u \rangle = 1467.14\,\mu m/s$; (c) sample 2, $\langle u \rangle = 4636.15\,\mu m/s$; (d) sample 1, $\langle u \rangle = 14671.36\,\mu m/s$. These figures are the same as those in Fig. 3(f)-(i) in the main text. (e)-(h) Flow field corresponding to the configurations (a)-(d), respectively. The flow proceeds from left to right.

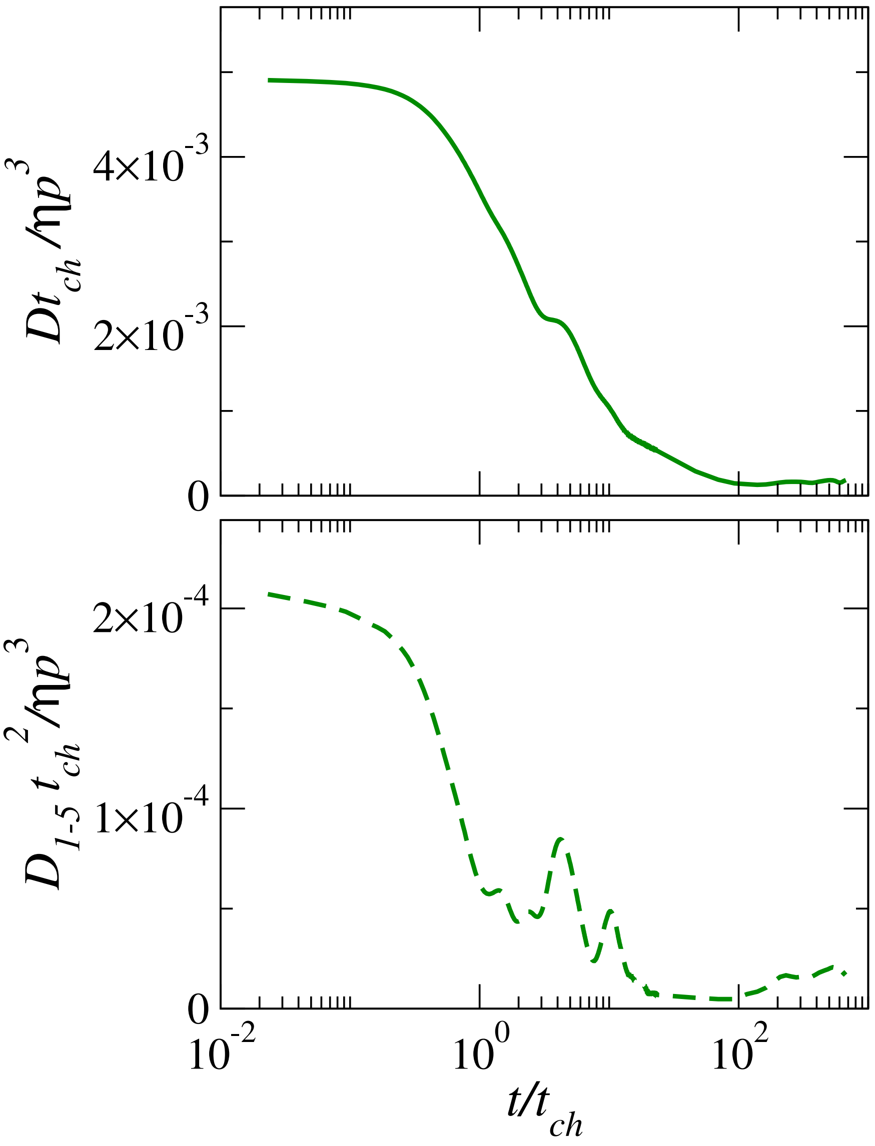


FIG. S7. Top: dissipation rate $D$ in Eq. 14 of the main text, as a function of time. Bottom: Dissipation rate $D_{1-5}$ given by the terms $\propto \alpha_1, \gamma_2, \alpha_4, (\alpha_5 + \alpha_6)$ in Eq. 14 of the main text, a functions of time. The average flow velocity $\langle u \rangle = 4636.15\,\mu m/s$ (sample 2, $t_{ch} \approx 0.002s$).

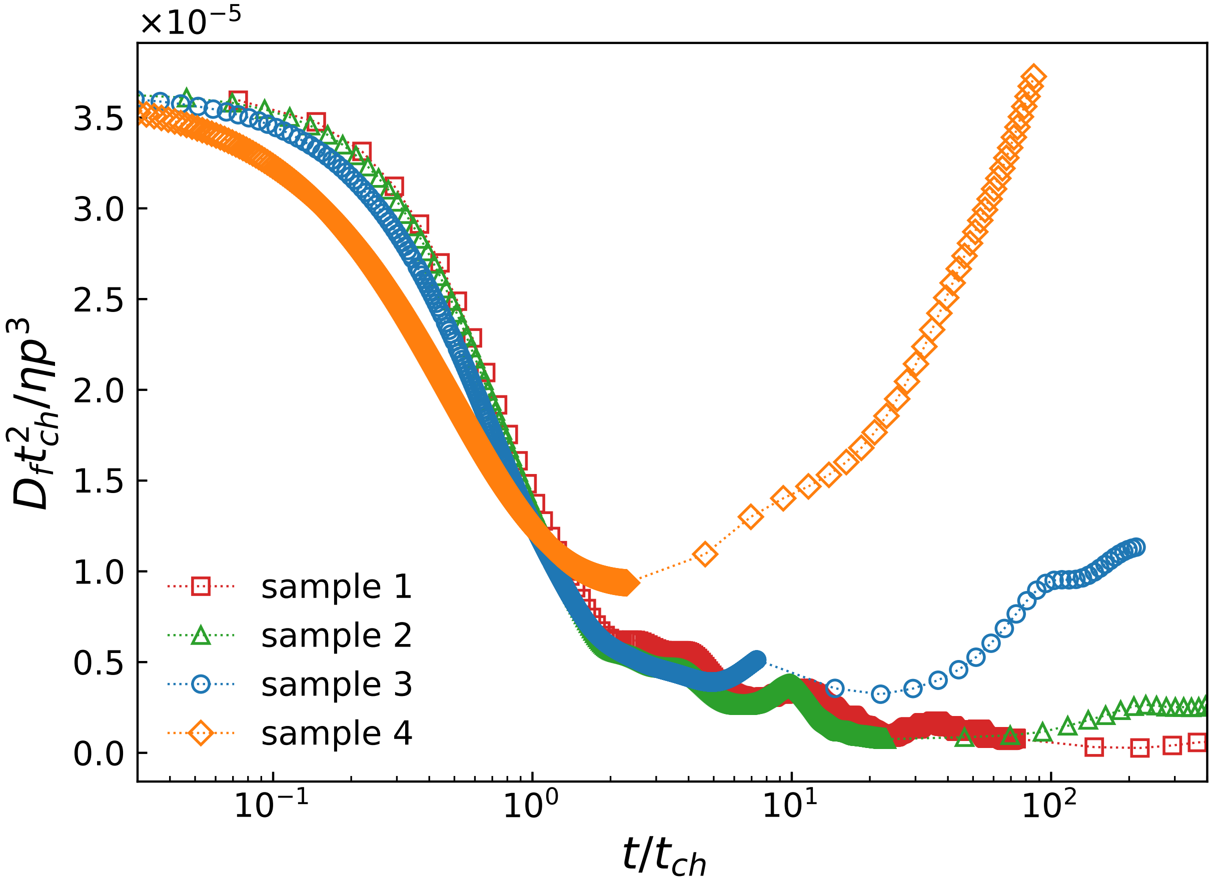


FIG. S8. Friction dissipation rate $D_f$ given by the term $\propto \chi-$ in Eq. 14 of the main text, defined as the excess over the friction dissipation rate of a uniform flow with velocity $\langle u \rangle$, as a function of time. Different symbols correspond to different flow velocities: sample 1 with $\langle u \rangle = 14671.36\,\mu m/s$ ($t_{ch} \approx 0.0007s$), sample 2 with $\langle u \rangle = 4636.15\,\mu m/s$ ($t_{ch} \approx 0.002s$), sample 3 with $\langle u \rangle = 1467.14\,\mu m/s$ ($t_{ch} \approx 0.007s$), and sample 4 with $\langle u \rangle = 463.62\,\mu m/s$ ($t_{ch} \approx 0.02s$).

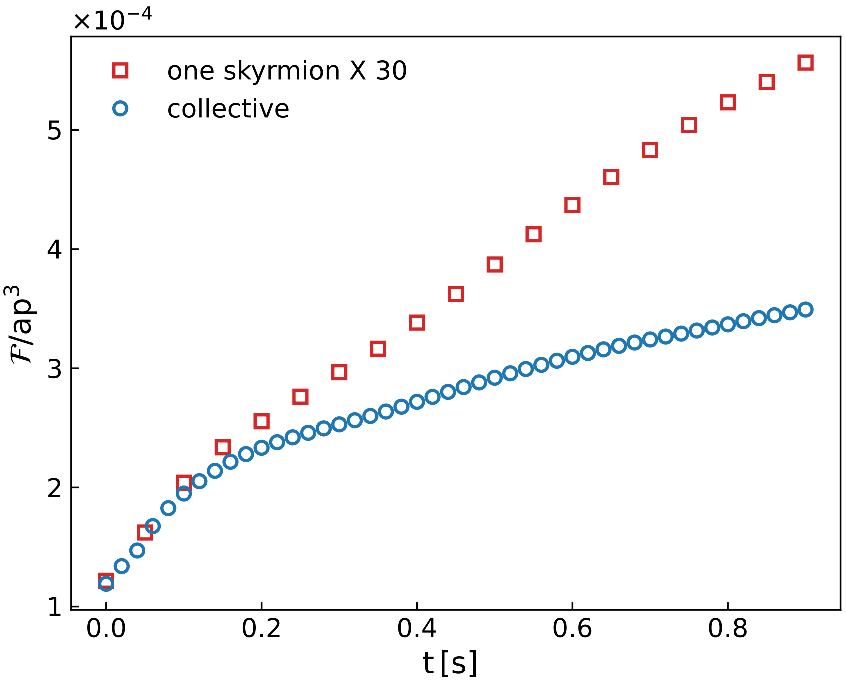


FIG. S9. Free energy of the system with 30 skyrmions (blue circles). The average velocity is that of sample 2, $\langle u \rangle = 4636.15\,\mu m/s$ ($t_{ch} \approx 0.002s$). The free energy of a single skyrmion in the same flow field (sample 2) is also shown (red squares).
